# Supplementary material for: Understanding How and Why University Students Use Virtual Private Networks
Source: arXiv:2002.11834 ancillary file (2021-02-22)

# Practicing Safe Browsing: Understanding How and Why University Students Use Virtual Private Networks

## Supplementary Materials


**1) INTERVIEW GUIDE** **2**

INTRODUCTION 2

General Privacy and Security Awareness 2

MAIN QUESTIONS 3

Past Experiences and Knowledge of VPNs 3

Current Usage of VPNs 3

Configuration 3

Privacy and Security 4

Strengths and Challenges of VPN Usage 5

Improvements to VPNs/General Privacy Enhancing Tools 5

CONCLUSION 5

**2) INTERVIEW SUMMARY CODEBOOK** **6**

**3) SURVEY QUESTIONS** **9**

Demographics 9

Privacy and Security Awareness 10

Privacy and Security Practices 12

VPN Perception 15

VPN Usage 25

VPN Utility 26

VPN Issues and Improvements 30

**4) ADDITIONAL SURVEY FIGURES: PARTICIPANTS THAT ONLY USED COMMERCIAL VPNS** **32**

Figure 1: Why do/did you use a VPN? (responses selected by participants) 32

Figure 13: Why do you think your VPN provider collects your data? (responses selected by participants) 33

Figure 14: What kind of data do you think your VPN provider collects about you? (responses selected by participants) 33

Figure 15: Who do you think has access to the data collected by your VPN? (responses selected by participants) 34

Figure 16: What information do you think is being shared with these entities? (responses selected by participants) 34

Figure 17: What do you think your VPN guarantees? (responses selected by participants) 35

# 1) INTERVIEW GUIDE

## INTRODUCTION

1. Introduce yourself
2. Thank the interviewee for their time
3. Explain what our project is about.
4. Mention that some questions may feel personal since we will ask about participant's experience and thoughts on VPN and that we can stop any time participant wishes to.
5. Present consent form – explain anonymity.
6. Ask for signatures: under the first part of the consent form and under permission to record.
7. Make sure the participant does not have any questions before you begin.
8. Start recording.
9. Ask some warm-up questions

### General Privacy and Security Awareness

**Data Practices**

1) What do you think censorship on the Internet is?
2) How do you feel about censorship on the Internet?
3) Is there online censorship in your home country? Tell me more about it.
4) What does the term online tracking mean to you?
5) Who do you believe is tracking you?
6) Why do you believe these entities are tracking you?

**Privacy**

7) Tell me about any tools you use to protect your privacy online or to overcome censorship

(Tracker blockers e.g. Privacy Badger, Ghostery, UBlock, Disconnect etc, Disable cookies on the browser, Private Browsing Mode, Tor Browser, Other)

8) How did you hear about these tools?
9) How long have you been using them?
10) Why do you use them?
11) Do you use these tools at the same time as your VPN? Why/Why not?

# MAIN QUESTIONS

## Past Experiences and Knowledge of VPNs

### Current Usage of VPNs

12) Tell me in your own words what a Virtual Private Network means to you?
13) If they do not use a VPN:
    a. What have you heard about Virtual Private Networks?
    b. Who/Where have you heard about VPNs from?
    c. Is there any reason for non-use of a VPN?
14) Why do you use a VPN?
15) When was the last time you used a VPN?
16) Are there any specific websites you visit using VPN?
    -Are they normally blocked or not?
17) Tell me about your first experience using a VPN
18) Can you recall how you learned about VPNs that you have used?
19) How would you explain what VPN does when you use it?
20) How do you feel about browsing while using a VPN?
    -How do you feel if you are not using a VPN?
21) Which VPNs have you used? (Show list if needed and ask participant to check all that apply or show you their phone/laptop if needed)

22) Where do you use VPN – home country, US, other?
23) Have you ever tried to create your own VPN? Why?
24) Can you tell me more about VPN usage in your country? Is there any issue with that?

## Configuration

25) What criteria do you use to assess if a VPN is trustworthy?
26) What is important for you when choosing a VPN provider?
27) Did you do anything to prepare your device for using VPN? (ex. enabling two-factor authentication, using browser extensions, IP-leak test) Why?
28) How do you feel about who the VPN service provider that you use is? Is that important for you? Why? Why not?
29) How do you check your VPN is connected/working?
30) Did you pay for your VPN? Why yes/not?
31) In your VPN do you have different countries you can choose to connect to?
32) Do you try to connect to any specific country? Which one and why?
33) Is the number of locations a VPN provider houses servers important for you? Why?(server network)
34) Did you get a clear description from your VPN provider of how to use VPN? Do you think it is needed/important? Why?

## Privacy and Security

35) Can you tell me about how your VPN providers explain how your privacy and security work while using VPN? Does your VPN provider explain it in a clear way?
36) Did you get an explanation of where your IP address is viewable? Where do you think it is?
37) Have you ever looked through your VPN provider's privacy policy? Any thoughts on that?

38) Do you think VPN guarantees you anonymity? What does it guarantee? What isn't guaranteed?
39) Do you think your VPN provider monitors or logs your activity? Why do you think so? What for?
40) Do you think your VPN provider's practices are transparent?
41) Do you think you can be tracked while using VPN? Tell me more.
42) Do you know whether your VPN provider shares any of your information? What do you think? If yes - what information? What about billing/payment info?
43) Do you think VPN should provide different levels of protection? Why? Why not? to whom?
44) Can you tell me more about how you feel when using VPN in terms of privacy and security?

## Strengths and Challenges of VPN Usage

45) Have you ever had any problems with a VPN?

- Tell me more

-How did you manage these issues?

46) Have you ever reported any issues to your VPN provider?
47) How would you describe your overall experience on Internet using VPN vs. not using VPN
48) Recall a time when you could not connect to VPN successfully. What did you think or feel?

## Improvements to VPNs/General Privacy Enhancing Tools

49) How would you improve a VPN?
50) What in your opinion a perfect VPN would provide?
51) Cheap/Fast/Secure - how would you list these 3 starting from the most important when choosing VPN and why?

52) Would you be willing to pay for a VPN subscription? -Why? - How much per month/year?

53) Would you trust a free VPN? Why?

54) Have you seen VPNs commercials? How often? Which VPNs?

55) Do you trust these commercials? Why? Why not?

## CONCLUSION

1. Ask the participant if there is anything s/he would like to add.
2. Explain what we are going to do with the data.
3. Ask for feedback.
4. Provide compensation or take details for compensation
5. Stop recording
6. Ask if the interviewee knows anyone else that wants to participate in the study
7. Thank the interviewee.

# 2) INTERVIEW SUMMARY CODEBOOK

| Main Code | Definition | Sub-Codes | Definition | Example quote and sub-code applied |
|---|---|---|---|---|
| Reasons for VPN usage | Reflects participants' motivations and goals behind VPN usage | Bypass geographic firewalls | Used to bypass location blocks | *"I have my mom reroute the US IP address to a Mexican IP address with a VPN, so then she could watch her Venezuelan TV shows."* P26<br>(Bypass geographic firewalls) |
| | | Work | Used for work purposes | |
| | | Privacy | Used to maintain privacy | |

| | | | | |
|---|---|---|---|---|
| | | Not Privacy/ Security | Used for neither privacy or security reasons | |
| What is a VPN? | Reflects participants‘ mental model of a VPN | Accessing blocked things | VPN enables accessing blocked content | *"It's sort of a middle man. So instead of you actually downloading the file from someplace where somebody might be looking at you downloading it, they download it for you and then they send it to your computer. So it figures that they downloaded it and not you."* P18<br><br>(Blocking IP address) |
| | | Blocking IP address | VPN enables changing and/or hiding user‘s IP address | |
| | | Another level of safety | VPN makes Internet usage more safe | |
| Guidelines when choosing VPN | Reflects participants‘ personal preferences of VPN's qualities and strategy in choosing a VPN | Good reputation | VPN has positive reviews | *"I look on, TechRadar and PC Monitor, those kinds of websites."* P11<br><br>(Good reputation) |
| | | Secure/Private | VPN is secure and provides privacy | |
| | | Ease of use | VPN's interface is user-friendly | |
| | | Speed | VPN does not slow down the Internet speed | |
| | | Cost | VPN has little or no cost | |
| | | Ease of set up | VPN is easy to set up | |
| Trust in VPN provider | Reflects participants‘ attitudes towards their VPN provider | Yes - Trust VPN | VPN is trustworthy | *"I feel very secure using it [University VPN]. But because it's affiliated to the university, I would definitely be more careful what I access on it. It's kind of like using a work computer. Definitely limiting myself strictly on university-affiliated sites. I think that I would be less careful if I had a VPN that wasn't university-affiliated"* P04 |
| | | No - Do not trust VPN | VPN is not trustworthy | |
| | | Reasons why trust/do not trust | Participant's explanation of why VPN is or is not trustworthy | |

| | | | | |
|---|---|---|---|---|
| | | View of importance of who provider is | Participant's explanation of whether they pay attention to who their VPN provider is | (View of importance of who provider is) |
| Using institution related VPN | Reflects participants' usage habits regarding institutional VPNs | Only for work | Institutional VPN used only for institution-related online activities | *"It really doesn't bother me if someone is looking at what I'm doing while I'm on the VPN"* P32<br><br>(Work + private browsing) |
| | | Work + private browsing | Institutional VPN used for both institution-related and personal online activities | |
| Use and trust free VPN | Reflects participants' attitudes towards commercial free VPNs | Yes - Trust free VPN | Free VPNs are trustworthy | *"If you're not paying for a service, it usually means that you are the service. (…) That's a terrible business model, but it's a free market. If people want to choose to trade their information in exchange for a free service, then that's their business, but I try not to."* P10<br><br>(No – Do not trust free VPN) |
| | | No - Do not trust free VPN | Free VPNs are not trustworthy | |
| | | Reasons why trust/do not trust free VPN | Participant's explanation of why free VPNs are or are not trustworthy | |
| VPN practices | Reflects participants' thoughts on VPNs' data practices | Keeping logs | Participants' thoughts on whether VPNs collect data about their users | *"If they share it with someone, then they're not sharing it in a way that I would be able to tell,"* P26<br><br>(Sharing information) |
| | | Sharing information | Participants' thoughts on whether VPNs send users' data to third parties | |
| What a VPN guarantees | Reflects participants' assumptions about VPNs' assertions | Anonymity | VPN provides online anonymity | *"If I use even a private VPN that I paid for, even though the majority of the world does not see my IP address and everything, I feel like the owners of the VPN provider will be able to still see it. And then it's just a* |
| | | Privacy | VPN protects privacy online | |

| | | | | |
|---|---|---|---|---|
| | | Access to websites | VPN provides access to all websites | *matter of having that security breached. So I don't think there's ever really a sense of true privacy. Unless I make my own VPN."* P04<br><br>(Nothing) |
| | | Nothing | Usage of VPN does not ensure anonymity, privacy, or accessing websites | |
| Tracking while using VPN | Reflects participants' assumptions about protection that VPNs provide against tracking | Yes - Tracking happens | VPNs do not ensure protection from tracking | *"Yes [I can be tracked while using a VPN], especially if I'm using the same IP address."* P21<br><br>(Yes – Tracking happens) |
| | | No - Tracking does not happen | VPNs ensure protection from tracking | |
| | | Views on who is tracking | Participant's reflection on what entities could be tracking VPN users | |

# 3) SURVEY QUESTIONS

## Demographics

Q2.1 What is your gender?

- O Male
- O Female

Q2.2 What is your age?

- O 18-25 years old
- O 26-35 years old
- O 36+ years old

Q2.3 What is your nationality?
▼ United States of America ... Kosovo

Display This Question: If 2.3 List of Countries = Other
Q2.3.1 If you selected "Other", what is your nationality?

______________________________________________________________

Display This Question: If 2.3 List of Countries = United States of America
Q2.4 What is your home state?
▼ Alabama ... I do not reside in the United States

Display This Question: If 2.3 List of Countries = All except United States of America
Q2.5 At what age did you move to the US?

- O Before 12 Before college
- O 13-17 Before college
- O 18-22 After college
- O 23-28 After college
- O 29-34 After college
- O 35+ After college

Q2.6 What is the highest level of education you are currently enrolled in or have completed?

- High school Undergraduate or lower
- Trade / technical / vocational school Undergraduate or lower
- Associate's (2-year) Undergraduate or lower
- Bachelor's (4-year) Undergraduate or lower
- Master's Post-undergraduate
- Doctorate Post-undergraduate
- Professional degree (JD, MBA, MD, etc) Post-undergraduate

Q2.7 What year are you completing in your program?

- N/A -- already completed
- 1st
- 2nd
- 3rd
- 4th
- 5th or greater

Q2.8 What is your field of study?
▼ African American Studies ... Other (specify below)

Display This Question: If 2.8 What is your field of study? = Other (specify below)
Q2.9 If you selected Other, what is your field of study?

________________________________________________________________

# Privacy and Security Awareness

Q3.1 Do you think any data is collected about you when you browse the Internet?

- Yes
- No

Display This Question: If 3.1 Do you think any data is collected about you when you browse the Internet? = Yes

Q3.2 Who do you think is collecting data about you? Check all that apply.

- ▢ My government Institution
- ▢ Other governments Institution
- ▢ My Internet Service Provider (ISP) Commercial
- ▢ My school Institution
- ▢ My employer Institution
- ▢ Friends and family Personal
- ▢ Companies Commercial
- ▢ Hackers Criminal
- ▢ Websites Commercial
- ▢ I don't know
- ▢ Other (specify) ________________________________________________

Display This Question: If 3.1 Do you think any data is collected about you when you browse the Internet? = Yes

Q3.3 Why do you think your data is being collected? Check all that apply.

- ▢ Political motives (i.e. identifying and influencing your political leanings)
- ▢ Advertising and other financial motives
- ▢ Crime investigation
- ▢ Theft (i.e. credit card info) Criminal
- ▢ Blackmail Criminal
- ▢ I don't know
- ▢ Other (specify) ________________________________________________

Display This Question: if 3.1 Do you think any data is collected about you when you browse the Internet? = Yes

Q3.4 What kind of data do you think is collected about you? Check all that apply.

- ☐ Location Metadata
- ☐ Demographics Metadata
- ☐ Interests / Preferences
- ☐ Online activities (websites visited, searches made, etc) Actions
- ☐ Private messages Actions
- ☐ Type of device you are using Metadata
- ☐ Recordings (microphone, webcam, screen capture, etc) Actions
- ☐ Keystrokes Actions
- ☐ I don't know
- ☐ Other (specify) ________________________________________________

Display This Question: if 3.1  Do you think any data is collected about you when you browse the Internet? = Yes

Q3.5 How concerned are you about this data collection?

- O Not at all concerned
- O Slightly concerned
- O Somewhat concerned
- O Moderately concerned
- O Extremely concerned

Display This Question: If 3.1 Do you think any data is collected about you when you browse the Internet? = No

Q3.6 Why not? Check all that apply.

- ☐ No one is collecting data
- ☐ I am not a person of interest
- ☐ I protect myself

☐ Other (specify) ________________________________________________

## Privacy and Security Practices

Q4.1 What tools and tactics have you used to protect yourself online? Check all that apply. Italicized numbers represent effort scores for each tool.

☐ Ad blocker 1

☐ Tracker blocker (eg. Ghostery) 2

☐ VPN 3

☐ Tor 3

☐ Private browsing (eg. Incognito Mode) 1

☐ Antivirus 1

☐ Deleting web history / cache / cookies / etc 1

☐ Avoiding submitting personal information online 1

☐ Turning off location services 1

☐ Avoiding spam emails 1

☐ Covering my webcam 1

☐ Using two-factor authentication (eg. SMS verification codes, Duo) 2

☐ Changing passwords frequently 2

☐ Using different passwords for each account 2

☐ Using a password manager 2

☐ Changing privacy settings on social media 2

- [ ] Avoiding making accounts (eg. social media) 3
- [ ] Checking website certificates / HTTPS 3
- [ ] Using different identities online
- [ ] Other (specify) ________________________________________________

Q4.2 Where did you hear about these tools and tactics? Check all that apply.

- [ ] Friends and family
- [ ] Employer Institution
- [ ] School Institution
- [ ] Online
- [ ] Other (specify) ________________________________________________

Q4.3 How long ago did you start using these tools and tactics?

- O < 6 months Past year
- O 6 months - 1 year Past year
- O 1-3 years
- O 3-5 years 3+ years
- O 5+ years 3+ years

Q4.4 When did you start using these tools and tactics?

- O Elementary school or earlier Before college
- O Middle school Before college
- O High school Before college
- O College College or later

- [ ] After college College or later

Q4.5 How often do you use these tools and tactics when you go online?

- [ ] Rarely
- [ ] Sometimes
- [ ] Most of the time
- [ ] Always

Q4.6 Where do you use these tools and tactics? Check all that apply.

- [ ] Public places
- [ ] Inside the US
- [ ] Outside the US
- [ ] Home
- [ ] Work Institution
- [ ] School Institution
- [ ] Other (specify) ____________________

Q4.7 On what devices do you use these tools and tactics? Check all that apply.

- [ ] Phone Mobile
- [ ] Tablet Mobile
- [ ] Laptop Computer
- [ ] Desktop Computer
- [ ] Other (specify) ____________________

## VPN Perception

Q5.1 In your words, what do you think a VPN is?

________________________________________________________________
________________________________________________________________
________________________________________________________________
________________________________________________________________
________________________________________________________________

Q5.2 How would you rate your knowledge about VPNs?

- O No knowledge
- O Some knowledge
- O High knowledge
- O Expert

Q5.3 Please check the types of VPN you have used below.

- ▢ VPN through my school Institutional
- ▢ VPN through my employer Institutional
- ▢ Paid commercial VPN
- ▢ Free commercial VPN
- ▢ Personal VPN (non-commercial VPN platform that I set up myself)
- ▢ Other (specify) ________________________________________________

Q5.4 Please select ALL paid commercial VPNs you have used. Note that some VPNs are listed under both paid and free. For this question, please only select VPNs where you have used the paid version.

- ▢ AceVPN
- ▢ AirVPN
- ▢ AzireVPN
- ▢ BlackVPN

- [ ] BolehVPN
- [ ] Buffered VPN
- [ ] CactusVPN
- [ ] CrypticVPN
- [ ] CRYPTOSTORM
- [ ] Doublehop
- [ ] ExpressVPN
- [ ] FinchVPN
- [ ] HeadVPN
- [ ] HIDE.ME
- [ ] HideIPVPN
- [ ] Hidester
- [ ] IBVPN
- [ ] IPREDATOR
- [ ] IPVanish
- [ ] IRONSOCKET
- [ ] IVPN
- [ ] Mullvad
- [ ] My Expat Network
- [ ] Newshosting

- [ ] NordVPN
- [ ] OctaneVPN
- [ ] OVPN
- [ ] Perfect Privacy
- [ ] Private Internet Access
- [ ] PrivateVPN
- [ ] ProtonVPN
- [ ] ProXPN
- [ ] Proxy.sh
- [ ] SaferVPN
- [ ] SecureVPN.to
- [ ] SEED4.ME
- [ ] ShadeYou VPN
- [ ] SlickVPN
- [ ] StrongVPN
- [ ] SunVPN
- [ ] SuperVPN
- [ ] SWITCHVPN
- [ ] Torguard
- [ ] TRUST.ZONE

- [ ] TunnelBear
- [ ] Tunnelr
- [ ] Unblock VPN
- [ ] VikingVPN
- [ ] VPN Land
- [ ] VPN.AC
- [ ] VPN.cc
- [ ] VPN.ht
- [ ] VPNArea
- [ ] VPNBaron
- [ ] VPNTunnel
- [ ] VyprVPN
- [ ] WhatTheServer
- [ ] Windscribe
- [ ] WorldVPN
- [ ] ZenMate
- [ ] ZoogVPN
- [ ] ZorroVPN
- [ ] Astrill VPN
- [ ] Encrypt.me

- [ ] F-Secure
- [ ] HideMyAss
- [ ] Hotspot Shield
- [ ] Private Tunnel
- [ ] HighVPN
- [ ] TigerVPN
- [ ] CyberGhost
- [ ] HolaVPN
- [ ] HiVPN
- [ ] Other (specify) ________________________________________________

Q5.5 Please select ALL free commercial VPNs you have used. Note that some VPNs are listed under both paid and free. For this question, please only select VPNs where you have used the free version.

- [ ] FinchVPN
- [ ] HIDE.ME
- [ ] Hotspot Shield
- [ ] ProtonVPN
- [ ] ProXPN
- [ ] SigaVPN
- [ ] TunnelBear
- [ ] VPNBaron

- [ ] Windscribe
- [ ] ZoogVPN
- [ ] Hola
- [ ] Onavo Protect
- [ ] SetupVPN
- [ ] HiVPN
- [ ] Betternet
- [ ] Other (specify) ________________________________________________

Display This Question: If 5.3 Please check the types of VPN you have used below. = VPN through my school Or 5.3 Please check the types of VPN you have used below. = VPN through my employer

Q5.6 How do you feel when using VPNs through your school and/or employer?

- O Vulnerable
- O Somewhat vulnerable
- O Neutral
- O Somewhat safe
- O Safe

Display This Question: If 5.4 Please select ALL paid commercial VPNs you have used Is Greater Than 0

Q5.7 How do you feel when using paid commercial VPNs?

- O Vulnerable
- O Somewhat vulnerable
- O Neutral
- O Somewhat safe
- O Safe

Display This Question: If 5.5 Please select ALL free commercial VPNs you have used Is Greater than 0

Q5.8 How do you feel when using free commercial VPNs?

- Vulnerable
- Somewhat vulnerable
- Neutral
- Somewhat safe
- Safe

Q5.9 Choose and rank the 5 most important factors for you when choosing a VPN.
Most important (in order)
______ Cost Accessibility
______ Speed Accessibility
______ Security Usage
______ Ease of setup / accessibility Accessibility
______ Ease of use Accessibility
______ Brand familiarity
______ Number of server locations Usage
______ Desired server location available Usage
______ Transparency Usage
______ Feature set Usage
______ Expert testimonial Brand
______ Online reviews Brand
______ Word of mouth Brand
______ Privacy Usage

Q5.10 For this question, please select the answer "Disagree".

- Strongly agree
- Agree
- Neutral
- Disagree
- Strongly disagree

Q5.11 Where did you hear about VPNs? Check all that apply.

- ☐ Friends and family

- ☐ Employer Institution
- ☐ Institution Institution
- ☐ Online
- ☐ Other (specify) ________________________________________________

Q5.12 How long ago did you first start using a VPN?

- O < 6 months Past year
- O 6 months - 1 year Past year
- O 1-3 years
- O 3-5 years 3+ years
- O 5+ years 3+ years

Q5.13 When did you first use a VPN?

- O Elementary school or earlier Before college
- O Middle school Before college
- O High school Before college
- O College College or later
- O After college College or later

Q5.14 Do you currently use a VPN?

- O Yes
- O No

Display This Question: If 5.14 Do you currently use a VPN? = No

Q5.15 Why did you stop using a VPN? Check all that apply.

- ☐ Too expensive Accessibility
- ☐ Not enough benefits Features
- ☐ Too hard to use Accessibility
- ☐ Internet speed too slow Accessibility
- ☐ I don't have anything to hide Perception
- ☐ I didn't use it enough Perception, Features
- ☐ It is not secure enough Perception, Features
- ☐ It didn't work Accessibility, Features
- ☐ I am no longer location restricted (e.g. using Hulu in a different country) Perception
- ☐ Other (specify) ________________________________________________

Q5.16 How often do/did you use a VPN when you go online?

- O Rarely
- O Sometimes
- O Most of the time
- O Always

Q5.17 Why do/did you use a VPN? Check all that apply.

- ☐ Protect my privacy
- ☐ Security
- ☐ Bypass Internet censorship Content access

☐ Recommended by friends or family Recommendation

☐ Recommended by expert Recommendation

☐ Access my institution's materials when away (university, workplace, etc) Content access

☐ Other (specify) ________________________________________________

Display This Question: If 5.17 Why do/did you use a VPN? Check all that apply. = Protect my privacy
Or 5.17 Why do/did you use a VPN? Check all that apply. = Security

Q5.18 Who are you trying to protect yourself from? Choose and rank your choices by your level of concern.

Most concerning (in order)
______ My government Institution
______ Other governments Institution
______ My Internet Service Provider (ISP) Commercial
______ My school Institution
______ My employer Institution
______ Friends and family
______ Companies Commercial
______ Hackers
______ Websites Commercial
______ Other (specify)

Q5.19 Where do/did you use a VPN? Check all that apply.

☐ Public places

☐ Inside the US

☐ Outside the US

☐ Home

☐ Work Institution

☐ School Institution

☐ Other (specify) ________________________________________________

Q5.20 On what devices do/did you use a VPN? Check all that apply.

☐ Tablet Mobile

- [ ] Phone Mobile
- [ ] Laptop Computer
- [ ] Desktop Computer
- [ ] Other (specify) ________________________________________________

# VPN Usage

Q6.1 How do you verify that your VPN is working? Please check all that apply. Italicized numbers represent effort scores for each method.

- [ ] My VPN alerts me (e.g. pop-up notification) 1
- [ ] I check that I can access normally blocked content 1
- [ ] My VPN has a "kill switch" that shuts off my connection when the VPN stops working 1
- [ ] My VPN displays ads while it is working 1
- [ ] I look at my VPN's icon in the status bar / task tray 2
- [ ] I check my IP address using my VPN 2
- [ ] I check my IP address using some tool other than my VPN 3
- [ ] I do not know how to verify that my VPN is working 0
- [ ] I do not verify that my VPN is working, even though I know how to do it -1
- [ ] Other (specify) ________________________________________________

Q6.2 Does your VPN offer servers in different locations?

- O Yes
- O No
- O I don't know

Q6.3 Do you have any preferences for any server locations? Please choose your preferred locations, if any. Hold the Cmd/Ctrl key to select multiple options.

▼ United States of America ... Kosovo

Q6.3.1 If you selected "Other", what other server locations do you prefer?
________________________________________________________________

Q6.4 What factors, if any, are important to you when choosing a server location? Please choose and rank them.
Important factors (in order)
______ Farther away from me
______ Closer to me Speed
______ Speed Speed
______ Internet freedom in host nation Nation
______ Stability in host nation Nation
______ Having access to desired content (e.g. Hulu)
______ Other (specify)

Q6.5 How did you learn how VPNs work? Check all that apply.

▢ VPN provider

▢ Friends and family

▢ Expert testimony Research

▢ Online research Research

▢ I do not know how they work

▢ Other (specify) ________________________________________________

# VPN Utility

Q7.1 Do you know how to see the server location of your VPN?

O Yes

O No

Q7.2 Do you know how to view the IP address provided by your VPN?

O Yes

O No

Q7.3 Did you read your VPN provider's privacy policy?

O Yes

O No

Q7.4 Do you think your VPN provider collects your data?

O Yes

O No

Display This Question: If 7.4 Do you think your VPN provider collects your data?= Yes
Q7.5 What data do you think your VPN provider collects? Check all that apply.

▢ Location Metadata

▢ Demographics Metadata

▢ Interests / Preferences

▢ Online activities (websites visited, searches made, etc) Actions

▢ Private messages Actions

▢ Type of device you are using Metadata

▢ Recordings (microphone, webcam, screen capture, etc) Actions

▢ Keystrokes Actions

▢ I don't know

▢ Other (specify) ________________________________________________

Display This Question: If 7.4 Do you think your VPN provider collects your data?= Yes
Q7.6 Why do you think your VPN collects your data? Check all that apply.

- [ ] Political motives (i.e. identifying and influencing your political leanings)
- [ ] Advertising and other financial motives
- [ ] It's a default consequence of being on the Internet
- [ ] Crime investigation
- [ ] Theft (i.e. credit card info) Criminal
- [ ] Blackmail Criminal
- [ ] I don't know
- [ ] Other (specify) ________________________________________________

Display This Question: if 7.4 Do you think your VPN provider collects your data?= Yes

Q7.7 Who do you think has access to the data collected by your VPN? Check all that apply.

- [ ] My government Institution
- [ ] Other governments Institution
- [ ] My Internet Service Provider (ISP) Commercial
- [ ] My school Institution
- [ ] My employer Institution
- [ ] Friends and family
- [ ] Companies Commercial
- [ ] Hackers
- [ ] Websites Commercial
- [ ] Only my VPN
- [ ] I don't know

☐ Other (specify) ________________________________________________

Display This Question: If 7.6 Why do you think your VPN collects your data? Check all that apply.= All except ‘Only my VPN’

Q7.8 What information do you think is being shared with these entities? Check all that apply.

☐ Location Metadata

☐ Demographics Metadata

☐ Interests / Preferences

☐ Online activities (websites visited, searches made, etc) Actions

☐ Private messages Actions

☐ Type of device you are using Metadata

☐ Recordings (microphone, webcam, screen capture, etc) Actions

☐ Keystrokes Actions

☐ I don't know

☐ Other (specify) ________________________________________________

Q7.9 For this question, please select the answer "Agree".

O Strongly agree

O Agree

O Neutral

O Disagree

O Strongly disagree

Q7.10 What do you think your VPN guarantees? Check all that apply.

☐ Anonymity Privacy

- ☐ Safety from tracking Security
- ☐ Access to content
- ☐ Blocking ads
- ☐ Masking my IP address Privacy
- ☐ Privacy Privacy
- ☐ I don't know
- ☐ Nothing
- ☐ Other (specify) ________________________________________________

Q7.11 How safe do you feel in terms of online privacy when using VPN?

- O Vulnerable
- O Somewhat vulnerable
- O Neutral
- O Somewhat safe
- O Safe

Q7.12 How safe do you feel in terms of online security when using VPN?

- O Vulnerable
- O Somewhat vulnerable
- O Neutral
- O Somewhat safe
- O Safe

## VPN Issues and Improvements

Q8.1 What issues, if any, have you run into when using a VPN? Check all that apply.

- ☐ It's not stable Ease
- ☐ It doesn't protect my privacy Perception, Features
- ☐ It isn't secure Perception, Features
- ☐ Some websites block VPNs Content
- ☐ Higher authority blocks my VPN (e.g. government) Content
- ☐ My VPN doesn't work Features, Content, Ease
- ☐ Complicated installation process Ease
- ☐ I don't understand how it works Ease
- ☐ I don't understand how to use it Ease
- ☐ I could not access the content I wanted Content
- ☐ Other (specify) ________________________________________________
- ☐ No issues

Q8.2 What do you like about your VPN(s)?

________________________________________________________________
________________________________________________________________
________________________________________________________________
________________________________________________________________
________________________________________________________________

Q8.3 What do you dislike about your VPN(s)?

________________________________________________________________
________________________________________________________________
________________________________________________________________
________________________________________________________________
________________________________________________________________

# 4) ADDITIONAL SURVEY FIGURES: PARTICIPANTS THAT ONLY USED COMMERCIAL VPNS

## Figure 1: Why do/did you use a VPN? (responses selected by participants)

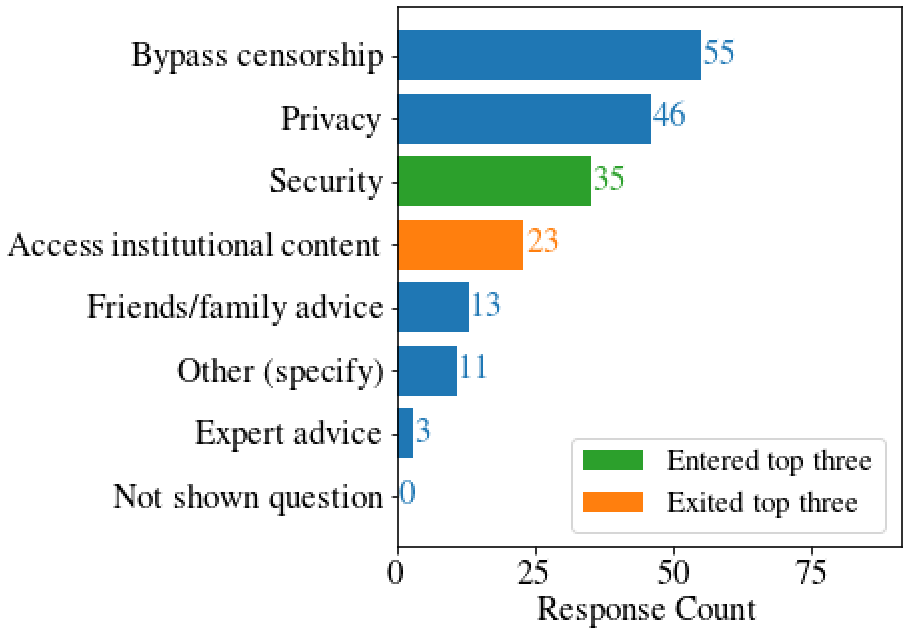

## Figure 13: Why do you think your VPN provider collects your data? (responses selected by participants)

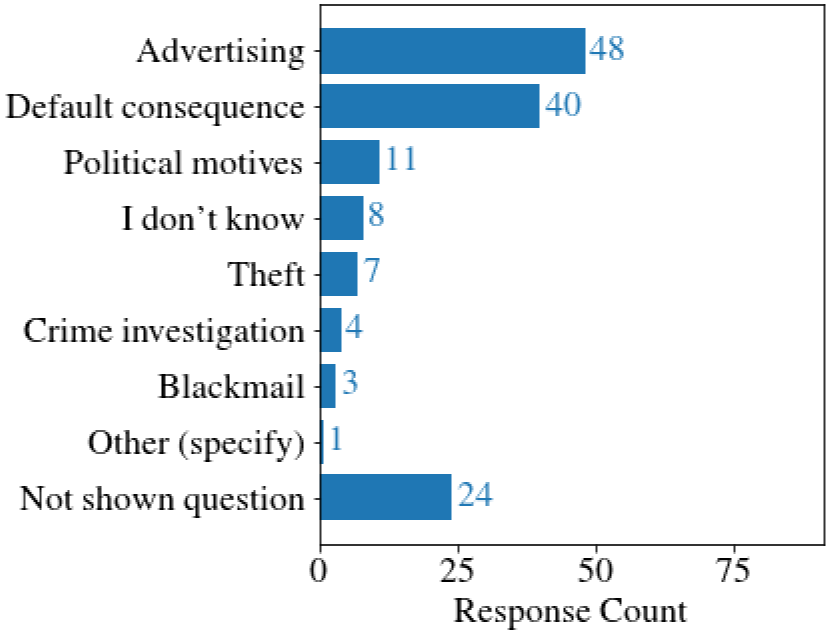

**Figure 14: What kind of data do you think your VPN provider collects about you? (responses selected by participants)**

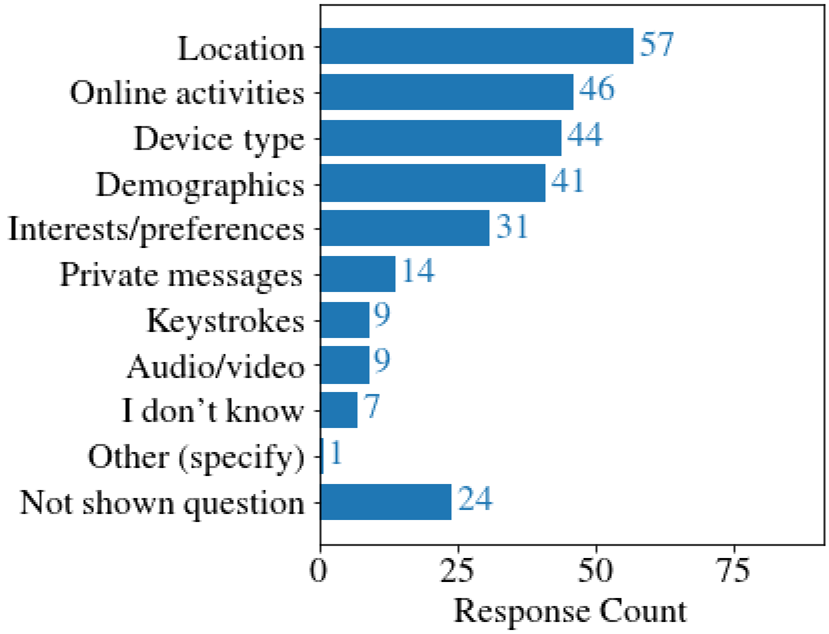

**Figure 15: Who do you think has access to the data collected by your VPN? (responses selected by participants)**

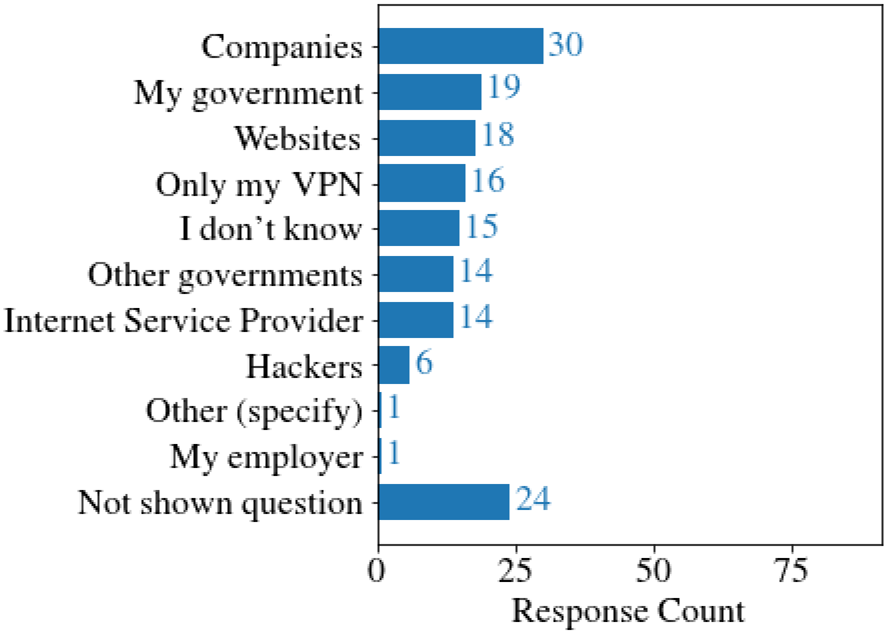

**Figure 16: What information do you think is being shared with these entities? (responses selected by participants)**

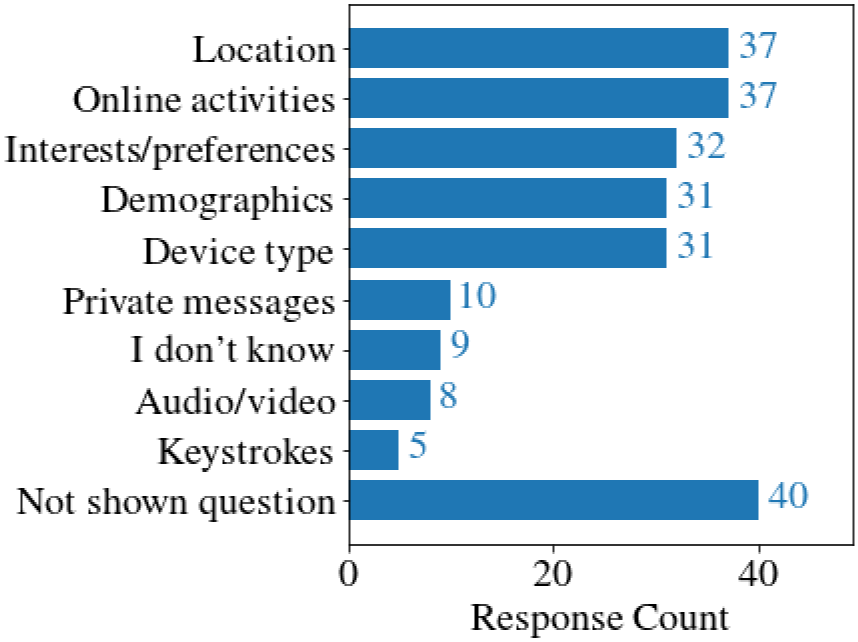

## Figure 17: What do you think your VPN guarantees? (responses selected by participants)

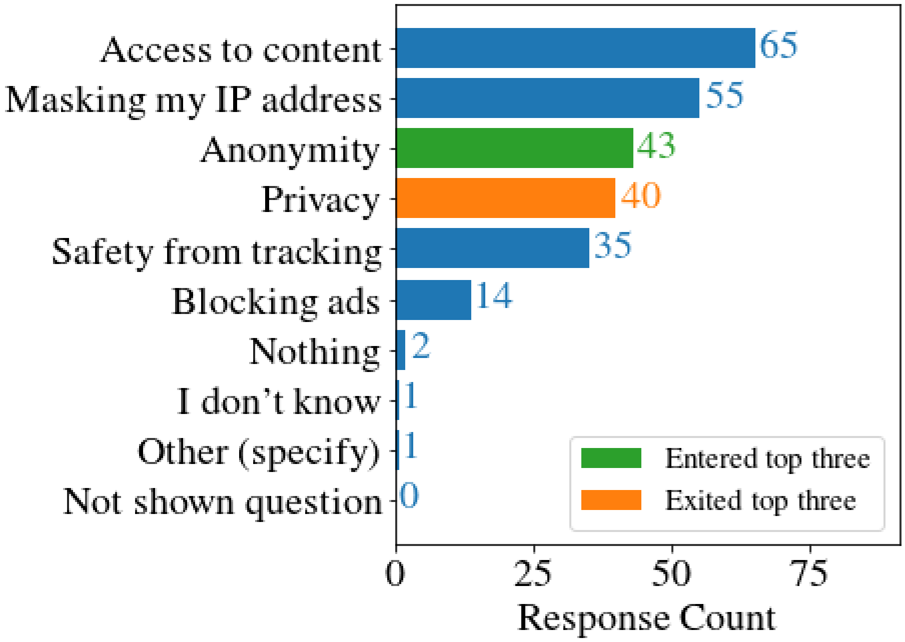

Supplement: Supplementary file 1 [file appendix.pdf]
