# Supplementary material for: Understanding How and Why University Students Use Virtual Private Networks
Source: arXiv:2002.11834 source file (2021-02-22)
Supplement: Supplementary file 2 [file appendix.tex]

\begin{appendix}
\section{Major Revision Changes}
    \subsection{Requested Changes}
    Our submission to the USENIX Security '20 Fall cycle was returned with a Major Revision decision. We rewrote the paper to address the reviewers' requested changes and more generally improve the results and paper. We addressed the following changes requested by reviewers:
    \begin{itemize}
        \item Included the codes for the interview portion of the study (Appendix).
        \item Improved the discussion of how the qualitative survey data was coded (Section 3.1.2).
        \item Included only counts (not percentages) for the frequency for any qualitative results so as not to suggest generalization of the results (Section 4).
        \item Add paragraph headings to present interview and survey results separately. For each section in the results, we presented the interview results first and then the survey results (Section 4).
        \item Separated results for students that only used university VPNs and students that have used commercial VPNs (Section 4).
        \item Expanded justification for why we focus on university students (Abstract, Section 1), and better articulated limitations of working with our group of university students (Section 3.3).
        \item Discussed statistical tests that were run that did not yield statistically significant results (Section 3.2.2).
        \item Removed the lab study from the paper.
    \end{itemize}

    \subsection{Additional Text Edits}
    As previously mentioned, we rewrote the paper to address the reviewers' requested changes.
    We list key changes to the text below:
    \begin{itemize}
        \item Pointed to future work in the introduction and conclusion.
        \item Emphasized the key takeaways in the abstract: "We found that students were mostly concerned with access to content, and privacy concerns were often secondary. They made tradeoffs to achieve a particular goal, such as using a free commercial VPN that potentially collects their online activities simply to access an online service in a geographically restricted area. Many users even expected that their VPNs were collecting data about them, although they did not understand how VPNs work."
        % \item Described why we focus on university students in the introduction and abstract
        \item Emphasized that we do not necessarily expect our results to generalize 
            beyond university students (Section 3.3).
        % \item Remove "Part 2" results section (the VPNAudit study), and remove VPNAudit-related text in abstract, intro, discussion, and conclusion
        % \item Listed the total number of participants and the number of participants that only used university-provided VPNs at the top of the results section
        % \item Present interview results first, then survey results.
        % \item Add paragraph headings to separate interview vs. survey results.
        \item Emphasized that students had many different factors they considered for choosing between VPNs (Section 4.3.2). We expected that privacy would be the main reason, but counter to our expectations, students had many expectations, e.g. cost and ease of use.
        \item Added Discussion section that summarizes key results and points to future work on making students more aware of the privacy risks of VPNs (Section 5).
        \item Used past tense when appropriate.
        \item Ensured that we provided both interview and survey data for each results section.
        \item Made all the citations in the References section look consistent.
        % \item Convert all percentages to counts when referring to groups of participants
        \item Removed a survey participant whose response to a particular question appeared to be a bug.
    \end{itemize}

    \subsection{Additional Figure Edits}
    As we rewrote the paper, we made several key changes to our figures and added new figures, which we list below:
    \begin{itemize}
        \item Indicated in figure captions whether responses for particular survey questions were coded by researchers or were multiple-choice.
        \item Added several figures for students that only used university-provided VPNs:
        \begin{itemize}
            \item Figure 1b: Why do/did you use a VPN?
            \item Figure 13b: Why do you think your VPN provider collects your data?
            \item Figure 14b: What kind of data do you think your VPN provider collects about 
        you?
            \item Figure 15b: Who do you think has access to the data collected by your VPN?
            \item Figure 16b: What information do you think is being shared with these entitites?
            \item Figure 17b: What do you think your VPN guarantees?
        \end{itemize}
        \item Added text explaining results for students that only used university-provided VPNs.
        \item When possible, put figures on each page in one row.
        % \item Color-coded "university VPN only" plots to highlight interesting results
        \item Only plotted responses for students that have used each respective type of VPN for Figure 12.
        \item Renamed 'No answer' label in y-axis to 'Not shown question' across figures.
        \item Added 'Did not answer' label in y-axis for Figures 10 and 11. Students could choose not to answer these two questions, but not other questions.
        \item Converted free responses for 'Other (please specify)' on Figures 10 and 11 to counts for different VPNs.
    \end{itemize}

    \begin{table*}[t]
    \centering
    \begin{tabular}{|c |l|} 
    \hline Main Code & Sub-codes \\
     \hline
    \multirow{6}{8em}{Reasons for VPN usage} &     \\
    & 1. Bypass geographic firewalls \\
    & 2. Work \\
    & 3. Privacy \\
    & 4. Not privacy/security 
    \\
    \hline
    \multirow{5}{8em}{What is a VPN?} &    \\
    & 1. Accessing blocked content  \\
    & 2. Blocking IP address  \\
    & 3. Another level of safety
    \\
    \hline
    \multirow{8}{8em}{Guidelines when choosing VPN} &    \\
    & 1. Good reputation \\
    & 2. Secure/Private \\
    & 3. Ease of use \\
    & 4. Speed \\
    & 5. Cost \\
    & 6. Ease of set up \\
    \hline
    \multirow{6}{8em}{Trust in VPN provider} &    \\
    & 1. Yes - Trust VPN \\
    & 2. No - Do not trust VPN \\
    & 3. Reasons why trust/do not trust \\
    & 4. View of importance of who provider is \\
    \hline
    \multirow{4}{8em}{Using institution related VPN} &    \\
    & 1.	Only for work \\
    & 2.	Work + private browsing \\
    \hline
    \multirow{5}{8em}{Use or trust free VPN} &    \\
    & 1.Yes - Trust free VPN \\
    & 2. No - Do not trust free VPN \\
    & 3. Reasons why trust/do not trust free VPN \\
    \hline
    \multirow{4}{8em}{VPN practices} &    \\
    & 1. Keeping logs \\
    & 2. Sharing information \\
    \hline
    \multirow{5}{8em}{What a VPN guarantees} &    \\
    & 1. Anonymity \\
    & 2. Privacy \\
    & 3. Access to websites \\
    \hline
    \multirow{5}{8em}{What a VPN does not guarantee} &    \\
    & 1. Anonymity \\ 
    & 2. Privacy \\ 
    & 3. Nothing \\
    \hline
    \multirow{5}{8em}{Tracking while using VPN} &    \\
    & 1. Yes - Tracking happens \\
    & 2. No - Tracking does not happen \\ 
    & 3. Views on who is tracking \\
     \hline
    \end{tabular}
    \caption{The summary of codes we used and reported, related to Interview portion of our study.}
    \label{table:3}
    \end{table*}
\end{appendix}
